# Supplementary material for: L00L entanglement and the twisted quantum eraser
Source: arXiv:2306.13620 source file (2023-10-17)
Supplement: Supplementary file 1 [file appendix.tex]

\section{appendix}

Let us assume we have two photons incident on beamsplitter. We can describe the input state as \cite{Brańczyk2017Hong-Ou-Mandel}:

\begin{equation}
    \left|\psi_{\text {in }}\right\rangle_{a b}=\adag_j \bdag_k |0\rangle_{a b}=|1 ; j\rangle_a|1 ; k\rangle_b
\end{equation}

The bottom indices are jsut to generalize for other properties to distinguish them and can be ignored for now (will be used later).

\medskip

Then, if our beamsplitter has reflectivity $r$ it affects our creation operators as: 

\begin{align}
    \adag &\stackrel{\hat{U}_{\mathrm{BS}}}{\longrightarrow} \sqrt{1-r} \adag +\sqrt{r} \bdag \\
    \bdag &\stackrel{\hat{U}_{\mathrm{BS}}}{\longrightarrow} \sqrt{r} \adag-\sqrt{1-r} \bdag
\end{align}

Which then gives our output state as:

\begin{equation}
    \begin{aligned}
    \left|\psi^{\text {out}}\right\rangle_{a b} & =\hat{U}_{\mathrm{BS}}\left|\psi^{\text {in }}\right\rangle_{a b} \\
    & =\left( \sqrt{r(1-r)} \adag_j \hat{a}_k^{\dagger}+r \hat{a}_k^{\dagger} \bdag_j-(1-r) \adag_j \bdag_k+\sqrt{r(1-r)} \bdag_j \bdag_k \right) |0\rangle_{a b}
    \end{aligned}
\end{equation}
\medskip

if r = 1/2 then we get:

\begin{equation}
    \left|\psi^{\text {out }}\right\rangle_{a b}=\frac{1}{2}\left(\adag_j \hat{a}_k^{\dagger}+\hat{a}_k^{\dagger} \bdag_j-\adag_j \bdag_k-\bdag_j \bdag_k\right)|0\rangle_{a b}
\end{equation}

Our state is then in a superposition of four equally probable outcomes, RR,TT,RT,TR.

We can now start adding properties to the photons j and k to distinguish them and see the interesting effects resulting from that. Particularly we want to see how it affects the coincidence probability, the probability to detect one photon in each mode/output of the beamsplitter

\subsubsection{Polarization}

Consider one photn in H and one in V (j = H, k = V)
We get our ouput to be:

\begin{align}
\left|\psi^{\text {out }}\right\rangle_{a b} & =\frac{1}{2}\left(\adag_H \adag_V+\adag_V \bdag_H-\adag_H \bdag_V-\bdag_H \bdag_V\right)|0\rangle_{a b} \\
& =\frac{1}{2}\left(|1 ; H\rangle_a|1 ; V\rangle_a+|1 ; V\rangle_a|1 ; H\rangle_b-|1 ; H\rangle_a|1 ; V\rangle_b-|1 ; H\rangle_b|1 ; V\rangle_b\right)
\end{align}

So, the coinidence probability (two middle terms) is $p=|1 / 2|^2+|-1 / 2|^2=1 / 2$. So, practically not much has changed.

Now lets consider indistinguishable photons, where $j=k=H$
Then now the state becomes:

\begin{equation}
    \begin{aligned}
    \left|\psi^{\text {out }}\right\rangle_{a b} & = \frac{1}{2} \left(\adag_H \adag_H+\adag_H \bdag_H-\adag_H \bdag_H-\bdag_H \bdag_H\right)|0\rangle_{a b} \\
    & = \frac{1}{2}\left(\adag_H \adag_H-\bdag_H \bdag_H\right)|0\rangle_{a b} \\
    & =\frac{1}{\sqrt{2}}\left(|2 ; H\rangle_a-|2 ; H\rangle_b\right) .
    \end{aligned}
\end{equation}

Now, because the photons are the same, we get destructive interference occurring between the middle terms such that we only have two possible outcomes, the photons bunch to either side. Note that we are still normalized as $\left(\adag\right)^n|0\rangle=\sqrt{n !}|n\rangle$
This is a two photon N00N state

\subsubsection{temporal distinguish-ability}
Now lets consider photons with different spectral/temporal such that we tune their time delays $\tau$ properties such as the figure below:

\begin{figure}[!h]
    \centering
    \includegraphics[width=0.7\textwidth]{temporal_distinguishable.png}
    \caption{temporal distinguish-ability \cite{Brańczyk2017Hong-Ou-Mandel}}
    \label{fig:timeline}
\end{figure}

To represent the spectral profile of the photon we can make use of the spectral amplitude function such that:

\begin{equation}
    |1 ; \phi\rangle_a=\int d \omega \phi(\omega) \adag(\omega)|0\rangle_a
\end{equation}

For two photons we get:

\begin{equation}
    \begin{aligned}
    \left|\psi^{\text {in }}\right\rangle_{a b} & =|1 ; \phi\rangle_a|1 ; \varphi\rangle_b \\
    & =\int d \omega_1 \phi\left(\omega_1\right) \adag\left(\omega_1\right) \int d \omega_2 \varphi\left(\omega_2\right) \bdag\left(\omega_2\right)|0\rangle_{a b}
    \end{aligned}
\end{equation}

We can now introduce a time delay such that: $\bdag(\omega) \rightarrow \bdag(\omega) \mathrm{e}^{-i \omega \tau}$. Then passing through a BS we get:

\begin{equation}
    \begin{aligned}
    \left|\psi^{\text {out }}\right\rangle_{a b}= & \hat{U}_{\mathrm{BS}}\left|\psi^{\mathrm{td}}\right\rangle_{a b} \\
    = & \frac{1}{2} \int d \omega_1 \phi\left(\omega_1\right)\left(\adag\left(\omega_1\right)+\bdag\left(\omega_1\right)\right) \int d \omega_2 \varphi\left(\omega_2\right)\left(\adag\left(\omega_2\right)-\bdag\left(\omega_2\right)\right) \mathrm{e}^{-i \omega_2 \tau}|0\rangle_{a b} \\
    = & \frac{1}{2} \int d \omega_1 \phi\left(\omega_1\right) \int d \omega_2 \varphi\left(\omega_2\right) \mathrm{e}^{-i \omega_2 \tau} \\
    & \times\left(\adag\left(\omega_1\right) \adag\left(\omega_2\right)+\adag\left(\omega_2\right) \bdag\left(\omega_1\right)-\adag\left(\omega_1\right) \bdag\left(\omega_2\right)-\bdag\left(\omega_1\right) \bdag\left(\omega_2\right)\right)|0\rangle_{a b} .
    \end{aligned}
\end{equation}

Now to calculate the coincidence probability we can model the detectors as having a flat frequency response and find the projectors for detection in each output:

\begin{equation}
    \begin{aligned}
        \hat{P}_a=\int d \omega \adag(\omega)\bra{0}_a \langle\left. 0\right|_a \hat{a}\left(\omega\right) \\
        \hat{P}_b ^=\int d \omega \bdag(\omega)|0\rangle_b\left\langle\left. 0\right|_b \hat{b}\left(\omega\right)
    \end{aligned}
\end{equation}

And so, using the density operator we find that the coincidence probability is:

\begin{equation}
    p=\operatorname{Tr}\left[\left|\psi^{\text {out }}\right\rangle_{a b}\left\langle\left.\psi^{\text {out }}\right|_{a b} \hat{P}_a \otimes \hat{P}_b\right]=\left\langle\left.\psi^{\text {out }}\right|_{a b} \hat{P}_a \otimes \hat{P}_b \mid \psi^{\text {out }}\right\rangle_{a b}\right.
\end{equation}

If we plug in the terms into the last equation and tidy up the equation we get to

\begin{equation}
    \begin{aligned}
    p_{\text {arb }}= & \frac{1}{4} \int d \omega_a \int d \omega_b \int d \omega_1 \int d \omega_2 \int d \omega_1^{\prime} \int d \omega_2^{\prime} \phi^*\left(\omega_1\right) \varphi^*\left(\omega_2\right) \phi\left(\omega_1^{\prime}\right) \varphi\left(\omega_2^{\prime}\right) \mathrm{e}^{i\left(\omega_2-\omega_2^{\prime}\right) \tau} \\
    & \times\left\langle\left. 0\right|_{a b}\left(\hat{a}\left(\omega_1\right) \hat{a}\left(\omega_2\right)+\hat{a}\left(\omega_2\right) \hat{b}\left(\omega_1\right)-\hat{a}\left(\omega_1\right) \hat{b}\left(\omega_2\right)-\hat{b}\left(\omega_1\right) \hat{b}\left(\omega_2\right)\right) \adag\left(\omega_a\right) \bdag\left(\omega_b\right) \mid 0\right\rangle_{a b} \\
    & \times\left\langle\left. 0\right|_{a b} \hat{a}\left(\omega_a\right) \hat{b}\left(\omega_b\right)\left(\adag\left(\omega_1^{\prime}\right) \adag\left(\omega_2^{\prime}\right)+\adag\left(\omega_2^{\prime}\right) \bdag\left(\omega_1^{\prime}\right)-\adag\left(\omega_1^{\prime}\right) \bdag\left(\omega_2^{\prime}\right)-\bdag\left(\omega_1^{\prime}\right) \bdag\left(\omega_2^{\prime}\right)\right) \mid 0\right\rangle_{a b}
    \end{aligned}
\end{equation}

Where the indices a and b are for the projectors Here the terms with odd numbers of operators in one mode go to zero while the other terms result in delta functions (since we only get 1 when the frequencies are the same):

\begin{equation}
    \begin{aligned}
    p_{\text {arb }}= & \frac{1}{4} \int d \omega_a \int d \omega_b \int d \omega_1 \int d \omega_2 \int d \omega_1^{\prime} \int d \omega_2^{\prime} \phi^*\left(\omega_1\right) \varphi^*\left(\omega_2\right) \phi\left(\omega_1^{\prime}\right) \varphi\left(\omega_2^{\prime}\right) \mathrm{e}^{i\left(\omega_2-\omega_2^{\prime}\right) \tau} \\
    & \times\left(\delta\left(\omega_2-\omega_a\right) \delta\left(\omega_1-\omega_b\right)-\delta\left(\omega_1-\omega_a\right) \delta\left(\omega_2-\omega_b\right)\right) \\
    & \times\left(\delta\left(\omega_2^{\prime}-\omega_a\right) \delta\left(\omega_1^{\prime}-\omega_b\right)-\delta\left(\omega_1^{\prime}-\omega_a\right) \delta\left(\omega_2^{\prime}-\omega_b\right)\right)
    \end{aligned}
\end{equation}

Finally, we can use the delta functions and the fac taht $\int d \omega|\phi(\omega)|^2=1$ to get:

\begin{equation}
    p_{\text {arb }}=\frac{1}{2}-\frac{1}{2} \int d \omega_1 \phi^*\left(\omega_1\right) \varphi\left(\omega_1\right) \mathrm{e}^{-i \omega_1 \tau} \int d \omega_2 \varphi^*\left(\omega_2\right) \phi\left(\omega_2\right) \mathrm{e}^{i \omega_2 \tau}
\end{equation}

Assuming the photons have the same spectral shape (only the timde delay is different) we get:

\begin{equation}
    p_{\text {arb}}=\frac{1}{2}-\frac{1}{2} \int d \omega_1\left|\phi\left(\omega_1\right)\right|^2 \mathrm{e}^{-i \omega_1 \tau} \int d \omega_2\left|\phi\left(\omega_2\right)\right|^2 \mathrm{e}^{i \omega_2 \tau}
\end{equation}

We can take this a step further and consider the photons to have gaussian spectral functions:

\begin{equation}
    \phi_i(\omega)=\frac{1}{(\pi)^{1 / 4} \sqrt{\sigma_i}} e^{-\frac{\left(\omega-\bar{\omega}_i\right)^2}{2 \sigma_i^2}} ; \quad(i=a, b)
\end{equation}
Then evaluating the integral via fourier transform the coincidence probability becomes:

\begin{equation}
    p_{\text {arb,gauss }}=\frac{1}{2}-\frac{\sigma_a \sigma_b}{\left(\sigma_a^2+\sigma_b^2\right)} e^{-\frac{\sigma_a^2 \sigma_b^2 \tau^2+\left(\bar{\omega}_a-\bar{\omega}_b\right)^2}{\sigma_a^2+\sigma_b^2}}
\end{equation}

If the Gaussians are the same then we get:

\begin{equation}
    p_{\text {arb,gauss }}=\frac{1}{2}-\frac{1}{2} \mathrm{e}^{-\frac{\sigma_a^2 \tau^2}{2}}
\end{equation}

So if the exponential goes to 1, i.e. if $\tau = 0$, then we get the the probability to be zero such that the photons bunch, as expected. reminder that $\sigma_a$ is the spectral width of the spectral amplitude function. A similar procedure can be done with sinc function to get: 

\begin{equation}
    p_{\text {arb,sinc }}=\frac{1}{2}-\frac{1}{8 A_a^2}\left(|\tau|-\left|\frac{\tau}{2}-A_a\right|-\left|\frac{\tau}{2}+A_a\right|\right)^2
\end{equation}

The difference betwee these two spectral amplitudes results in a different shape of HOM dip

\medskip

For entangled photons we need t oconsider the Joint-spectral amplitude instead:

\begin{equation}
    \left|\psi^{\text {in }}\right\rangle_{a b}=\int d \omega_1 \int d \omega_2 f\left(\omega_1, \omega_2\right) \adag\left(\omega_1\right) \bdag\left(\omega_2\right)|0\rangle_{a b}
\end{equation}

With the same procedure as before we can apply a time delay to one of the modes, then act with the beam splitter unitary transformation, then we calculate the coincidence probability with the projectors. This yields the coincidence probability:

\begin{equation}
    p_{\text {ent }}=\frac{1}{2}-\frac{1}{2} \int d \omega_1 \int d \omega_2 f^*\left(\omega_1, \omega_2\right) f\left(\omega_2, \omega_1\right) \mathrm{e}^{i\left(\omega_2-\omega_1\right) \tau}
\end{equation}

since the JSA of entangled photons is typically not seperable: $f\left(\omega_1, \omega_2\right) \neq \phi\left(\omega_1\right) \varphi\left(\omega_2\right)$

This expression can also be expressed in its Schmidt decomposition which results in:

\begin{equation}
    p_{\text {ent }}=\frac{1}{2}-\frac{1}{2} \sum_{k, k^{\prime}} u_k u_{k^{\prime}} \int d \omega_1 \phi_k^*\left(\omega_1\right) \varphi_{k^{\prime}}\left(\omega_1\right) \mathrm{e}^{-i \omega_1 \tau} \int d \omega_2 \varphi_k^*\left(\omega_2\right) \phi_{k^{\prime}}\left(\omega_2\right) \mathrm{e}^{i \omega_2 \tau}
\end{equation}

\section{HOM dip with l-states}

We want to consider how the HOM dip where one input state has been transformed by an l phase plate. We thus need to expand our basis to include a spatial mode basis with two diffeten l modes, $l_1 andl_2$. We therefore have We assume here that both incoming photons are polarized in the same direction and that we have the possibility of inducing a optical path length difference in the in put state. Thus we get input state:

\begin{equation}
    \left|\psi_{\text {in }}\right\rangle_{a b} = \adag_{l_1} \bdag_{l_2}|0\rangle_{a b}=|1 ; {l_1}\rangle_a|1 ; {l_2}\rangle_b
\end{equation}

Since the beamsplitter does not affect the spatial profile of the beams we get the same result as teh first section where it operates on each input direction as:

\begin{align}
    \adag &\stackrel{\hat{U}_{\mathrm{BS}}}{\longrightarrow} \sqrt{1-r} \adag+\sqrt{r} \bdag \\
    \bdag &\stackrel{\hat{U}_{\mathrm{BS}}}{\longrightarrow} \sqrt{r} \adag-\sqrt{1-r} \bdag
\end{align}

Which then gives our output state as:

\begin{equation}
    \begin{aligned}
    \left|\psi^{\text {out }}\right\rangle_{a b} & =\hat{U}_{\mathrm{BS}}\left|\psi^{\text {in }}\right\rangle_{a b} \\
    & =\hat{U}_{\mathrm{BS}}\left(\adag_{l_1} \bdag_{l_2}|0\rangle_{a b}\right) \\
    & =\left(\sqrt{1-r} \adag_{l_1}+\sqrt{r} \bdag_{l_1}\right)\left(\sqrt{r} \adag_{l_2}-\sqrt{1-r} \bdag_{l_2}\right)|0\rangle_{a b} \\
    & =\left(\sqrt{r(1-r)} \adag_{l_1} \adag_{l_2}+r \adag_{l_2} \bdag_{l_1}-(1-r) \adag_{l_1} \bdag_{l_2}+\sqrt{r(1-r)} \bdag_{l_1} \bdag_{l_2}\right)|0\rangle_{a b} .
    \end{aligned}
\end{equation}

again, assuming r = 1/2 we get:

\begin{equation}
    \left|\psi^{\text {out }}\right\rangle_{a b}=\frac{1}{2}\left(\adag_{l_1} \adag_{l_2}+\adag_{l_2} \bdag_{l_1}-\adag_{l_1} \bdag_{l_2}-\bdag_{l_1} \bdag_{l_2}\right)|0\rangle_{a b}
\end{equation}

Writing the beamsplitter as a 4x4 matrix where our basis is $\left(\adag_{l_1},\bdag_{l_1},\adag_{l_2},\bdag_{l_2}\right)^T$ we find:

\begin{equation}
\hat{U}_{BS} = \frac{1}{\sqrt{2}} \begin{pmatrix}
1 & 1 & 0 & 0 \\
1 & -1 & 0 & 0 \\
0 & 0 & 1 & 1 \\
0 & 0 & 1 & -1 \\
\end{pmatrix}
\end{equation}

We now want to interfere our l-modes. We can model our SLM exactly as the beamsplitter but instead of interfering the a and b modes we interfere the l modes with some "reflectivity and "transmission". lets call them $s$ and $t$ respectively. As opposed to the the beamsplitter which is a 50:50, the SLMs parameters can be altered, phase and amplitude, however, we require that $|r|^2 + |t|^2 = 1$ since we want our matrix to be unitary (lossless). The operation of the SLM is then:

\begin{align}
    l_1 &\stackrel{\hat{U}_{\mathrm{SLM}}}{\longrightarrow} tl_1+ rl_2 \\
    l_2 &\stackrel{\hat{U}_{\mathrm{SLM}}}{\longrightarrow} rl_1+tl_2 \\
\end{align}

here $t = |t|\exp{i\theta}, r = |r|\exp{i\phi}$. From the fact that the matrix is unitary and the absolute squares add to 1 we can constrict our matrix to have only 1 parameter (ignoring global phase) such that:

\begin{align}
    l_1 &\stackrel{\hat{U}_{\mathrm{SLM}}}{\longrightarrow} \cos(\theta)l_1+ i\sin(\theta)l_2 \\
    l_2 &\stackrel{\hat{U}_{\mathrm{SLM}}}{\longrightarrow} i \sin(\theta)l_1+ \cos(\theta)l_2 \\
\end{align}

Here theta is the angle between t and r. So, we get:

\begin{equation}
    \hat{U}_{SLM} = \begin{pmatrix}
    \cos(\theta) & 0 & i\sin(\theta) & 0 \\
    0 & \cos(\theta) & 0 & i\sin(\theta) \\
    i\sin(\theta) & 0 & \cos(\theta) & 0 \\
    0 & i\sin(\theta) & 0 & \cos(\theta) \\
    \end{pmatrix}
\end{equation}

S our final matrix will become:
\begin{equation}
     \hat{U}_{SLM}\hat{U}_{BS} =\frac{1}{\sqrt{2}}  \left(\begin{array}{cccc}
    \cos (\theta) & \cos (\theta) & i \sin (\theta) & 0 \\
    \cos (\theta) & -\cos (\theta) & i \sin (\theta) & -i \sin (\theta) \\
    i \sin (\theta) & i \sin (\theta) & \cos (\theta) & 0 \\
    i \sin (\theta) & -i \sin (\theta) & \cos (\theta) & -\cos (\theta)
    \end{array}\right)
\end{equation}

\subsection{two photon detection space}

If we want to simulate the results we expect from experimentation then we must bring our matrix from the 1 photon space with 4 modes to two photon space: Boson Sampling.

\newpage

\begin{begin}
    P_a &\stackrel{\hat{U}_{\mathrm{SLM}}}{\longrightarrow} c_1\ket{l_1} + c_2\ket{l_2} \\
\end{begin}

$\left(\adag_{l_1},\bdag_{l_1}\adag_{l_2},\bdag_{l_2}\right)^T$

\subsection{HOM effect}
The well-studied Hong-Ou-Mandel effect is one of the most notable examples of quantum interference. This simple and elegant theory describes the very curious wave-particle duality behaviour one observe when two indistinguishable photons interfere on a beamsplitter (BS).

\medskip 

If one considers 2 photons incident on the the input ports to a 50:50 BS, the operation of the beamsplitter on the photons can be described in terms of the creation operators $\adag,\bdag$ as:

\begin{equation}
    \adag &\stackrel{\hat{U}_{\mathrm{BS}}}{\longrightarrow} \frac{1}{\sqrt{2}}\left( \adag + \bdag \right) ,  \quad\quad \bdag &\stackrel{\hat{U}_{\mathrm{BS}}}{\longrightarrow} \frac{1}{\sqrt{2}}\left( \adag - \bdag \right)
\end{equation}

\begin{eqnarray}\label{eq:HOM-1}
	\adag\bdag\ket{0} \quad\xrightarrow{BS}\quad \frac{1}{2} \left( \adag + \bdag \right) \left( \adag - \bdag \right)\ket{0}
	\quad=\quad\frac{1}{\sqrt{2}}\left( \ket{2_a,0}+\ket{0,2_b} \right)
\end{eqnarray}

Note here that the state normalizes as$ \left(\adag\right)^n\ket{0}=\sqrt{n!}\ket{n}$. meaning 2 photons are in mode $a$ or 2 photons are in mode $b$, but there is \textbf{never} one photon in mode $a$ and at the same time one photon in $b$. Often referred to as photon bunching. This quantum interference, however, only occurs when our photons are indistinguishable. If we instead consider photons distinguishable in some other degree of freedom, which we refer to as $j$ and $k$ then we do not see any interference and our state reads instead:

\begin{eqnarray}\label{eq:HOM-dist}
    \adag_j\bdag_k\ket{0}\xrightarrow{BS} \frac{1}{2} \left( \adag_j +       \bdag_j \right) \left( \adag_k - \bdag_k \right)\ket{0} = \frac{1}{2} \left( \adag_j \adag_k + \adag_k \bdag_j - \adag_j \bdag_k - \bdag_j \bdag_k \right)\ket{0},
\end{eqnarray}

For the sake of readability we omit the ``hat'' of the operator and write the OAM value in brackets after the operator $\text{a}^{\dagger }(\ell)$. Thus the SPDC state now reads, only $\ell\in\{-1,0,1\}$ is considered for simplicity
\begin{equation}
	\ket{\psi_{\text{SPDC}}}=\Big[\text{a}^{\dagger }(-1).\text{b}^{\dagger }(1)+\text{a}^{\dagger }(0).\text{b}^{\dagger }(0)+\text{a}^{\dagger }(1).\text{b}^{\dagger }(-1)\Big]\ket{0}.
\end{equation}
Adding a mirror in path A flips the OAM sign in this path (see section~\ref{sec:linear_optical_elements_to_manipulate_photons})
\begin{equation}
	\ket{\psi_{\text{SPDC}}}\xrightarrow{M(a)}\Big[\text{a}^{\dagger }(-1).\text{b}^{\dagger }(-1)+\text{a}^{\dagger }(0).\text{b}^{\dagger }(0)+\text{a}^{\dagger }(1).\text{b}^{\dagger }(1)\Big]\ket{0},
\end{equation}
where the overall $i$ phase is omitted. Sending this state onto a beam splitter as depicted in Fig.~\ref{fig:HOM-setups}~b) yields
\begin{eqnarray}
	\ket{\psi_{\text{SPDC}}}\xrightarrow{\text{BS}\cdot\text{M(a)}}\frac{1}{2} \Big(-i \text{a}^{\dagger }(-1).\text{b}^{\dagger }(-1)-i \text{a}^{\dagger }(0).\text{b}^{\dagger }(0)-i \text{a}^{\dagger }(1).\text{b}^{\dagger }(1)\\\nonumber
	+i \text{b}^{\dagger }(-1).\text{a}^{\dagger }(-1)+i \text{b}^{\dagger }(0).\text{a}^{\dagger }(0)+i \text{b}^{\dagger }(1).\text{a}^{\dagger }(1)\\\nonumber
	-\text{a}^{\dagger }(-1).\text{a}^{\dagger }(1)-\text{a}^{\dagger }(0).\text{a}^{\dagger }(0)-\text{a}^{\dagger }(1).\text{a}^{\dagger }(-1)\\\nonumber
	-\text{b}^{\dagger }(-1).\text{b}^{\dagger }(1)-\text{b}^{\dagger }(0).\text{b}^{\dagger }(0)-\text{b}^{\dagger }(1).\text{b}^{\dagger }(-1)\Big)\ket{0}.
\end{eqnarray}
Considering $\ell=0$ photons only, then the same result as previously calculated occurs. This means that ``filtering'' the correct terms yields also the HOM type interference. For example, applying an SLM operation of $\text{SLM}(-1)$ and additionally using a single mode fiber SMF in both arms A and B results in selecting only modes where $\ell=1$ in both modes
\begin{equation}
	\ket{\psi_{\text{SPDC}}}\xrightarrow{\text{SMF}\cdot\text{SLM}(-1)\cdot\text{BS}\cdot\text{M(a)}}\frac{1}{2} \left(-i \text{a}^{\dagger }(1).\text{b}^{\dagger }(1)+i \text{b}^{\dagger }(1).\text{a}^{\dagger }(1)\right)\ket{0}.
\end{equation}
Note that although technically the above state should have $\ell=0$ everywhere because the photons are physically in this state, here they are written with $\ell=1$ to make it clear that the interference happened between these modes. The projection into $\ell=0$ mode with the SLM and the SMF is only to post-select these events. It should be stressed that in any experimental configuration one relies on this kind of selection, also in the $\ell=0$ case. Therefore, to observe the desired HOM interference the commutator between these two terms $\Big[\text{a}^{\dagger }(1),\text{b}^{\dagger }(1)\Big]$ must vanish. This is accomplished by overlapping the two photons perfectly in the spatial and temporal domain. The spatial domain is addressed by careful alignment of the incoming beams at the beam splitter, while the temporal domain is dependent on the spectral bandwidth as well as on the arrival time of the two photons at the beam splitter. A trombone system and narrow bandpass filters, as depicted in Fig.~\ref{fig:HOM-setups}~b), are used to ensure the temporal overlap. This very same procedure also applies to higher order $\ell$ modes and is demonstrated experimentally, see section~\ref{sec:experimental_results_HOM-dips-one-crystal}.

In Fig.~\ref{fig:HOM-setups}~c) another experimental setup is shown. This setup contains an additional spiral phase plate (SPP). For simplicity let us consider here only the $\ell=0$ modes emitted by the ppKTP crystal. Then the SPP adds an OAM value of $\ell=2$ in arm A to the state and then we apply the beam splitter operation, thus the state reads
\begin{equation}
	\frac{1}{2} \left(-\text{a}^{\dagger }(-2).\text{b}^{\dagger }(0)+\text{b}^{\dagger }(2).\text{a}^{\dagger }(0)+i \text{a}^{\dagger }(-2).\text{a}^{\dagger }(0)+i \text{b}^{\dagger }(2).\text{b}^{\dagger }(0)\right)\ket{0}
\end{equation}
and after another reflection in arm A
\begin{equation}
	\frac{1}{2} \left(-i \text{a}^{\dagger }(2).\text{b}^{\dagger }(0)+i \text{b}^{\dagger }(2).\text{a}^{\dagger }(0)-\text{a}^{\dagger }(2).\text{a}^{\dagger }(0)-\text{b}^{\dagger }(2).\text{b}^{\dagger }(0)\right)\ket{0}.
\end{equation}
Since only coincidence events between detector A and B are detected, the state can be written as
\begin{equation}
	\ket{\chi}=\frac{1}{\sqrt{2}}\Big(\ket{0,2}-\ket{2,0}\Big),
\end{equation}
where the state is properly renormalized. Measuring in the superposition $\ket{0}+\ket{2}$ on both detectors yield a minimum and hence a HOM interference like previously observed is expected. On the contrary, measuring $\ket{0}+\ket{2}$ on detector A and $\ket{0}-\ket{2}$ on detector B yields a maximum, thus resulting in the observation of a HOM interference bump. The expectation value of an operator $\mathcal{P}_{\text{bump}}$ with
\begin{eqnarray}
	\mathcal{P}_{\text{bump}}=\frac{1}{4}(\ket{0}+\ket{2})_A(\bra{0}+\bra{2})_A\otimes(\ket{0}-\ket{2})_B(\bra{0}-\bra{2})_B\\\nonumber
	=\frac{1}{4}\Big(\ketbra{00}{00}+\ketbra{20}{00}+\ketbra{00}{20}+\ketbra{20}{20}\\\nonumber
	-\ketbra{02}{00}-\ketbra{22}{00}-\ketbra{02}{20}-\ketbra{22}{20}\\\nonumber
	-\ketbra{00}{02}-\ketbra{20}{02}-\ketbra{00}{22}-\ketbra{20}{22}\\\nonumber
	\ketbra{02}{02}+\ketbra{22}{02}+\ketbra{20}{22}+\ketbra{22}{22}\Big).
\end{eqnarray}
Thus the expectation value of $\mathcal{P}_{\text{bump}}$ is
\begin{equation}
	\bra{\chi}\mathcal{P}_{\text{bump}}\ket{\chi}=\frac{1}{2}.
\end{equation}
Note that for a mixed state $\rho_\chi$ we would expect
\begin{equation}
 	\text{Tr}\big(\rho_\chi \mathcal{P}_{\text{bump}}\big)=\frac{1}{4},
 \end{equation} 
 
with $\rho_\chi=\frac{1}{2}\Big(\ketbra{02}{02}+\ketbra{20}{20}\Big)$. This shows that an expectation value of $\frac{1}{2}$ is indeed a bump with double the expectation value as compared to a mixed state.
Additionally, a detailed calculation shows that higher order $\ell$ terms produced in the SPDC process do not interfere with the derivation shown here. Furthermore, the SPP could take any arbitrary value of $\ell$, thus the scheme presented here is a method to create arbitrary states of the from
 
\begin{equation}
 	\ket{\chi_\ell}=\frac{1}{\sqrt{2}}\Big(\ket{\ell,0}-\ket{0,\ell}\Big),
 \end{equation} 
conditioned on coincidence-events between detector A and B. These states are called $\ell 00\ell$-states.

\begin{equation}
     \hat{U}_{SLM}\hat{U}_{BS}\left|\psi_{\text {in }}\right\rangle_{a b} =\frac{1}{\sqrt{2}}  \left(\begin{array}{c}
    \cos (\theta) \\
    \cos (\theta)-i \sin (\theta) \\
    i \sin (\theta) \\
    i \sin (\theta)-\cos (\theta)
    \end{array}\right)
\end{equation}
